# Supplementary material for: Future Transformer for Long-term Action Anticipation
Source: arXiv:2205.14022 source file (2022-05-27)
Supplement: Supplementary file 1 [file Sup_Figure_query.tex]

\begin{figure}[t]
    \centering
    \includegraphics[width=\linewidth]{Figures/Supplementary/query.pdf}
\caption{\textbf{query.} }
\label{fig:query}
\vspace{-4mm}
\end{figure}
